# Supplementary material for: FLAIRS: FPGA-Accelerated Inference-Resistant & Secure Federated Learning
Source: arXiv:2308.00553 source file (2023-08-01)
Supplement: Supplementary file 1 [file 99_appendix.tex]

\subsection{\flame}
\label{subsec:flame}
\noindent The backdoor-aware \flame consists of three defense layers (outlier-detection-based filtering, clipping, adding noise). The rationale here is that a sufficiently high noise can remove the backdoor but will also drop the models' utility in terms of accuracy on the main task. The filtering and clipping mitigate backdoored models that would require a high amount of noise, allowing \flame to mitigate the remaining poisoned models with a low noise level, causing only a tolerable drop of the MA. Its overall structure is shown in Fig.~\ref{fig:flame}.

\begin{figure}[b]
    \centering
    \includegraphics[width=0.8\linewidth,trim={0cm 0cm 0.0cm 4.65cm},clip]{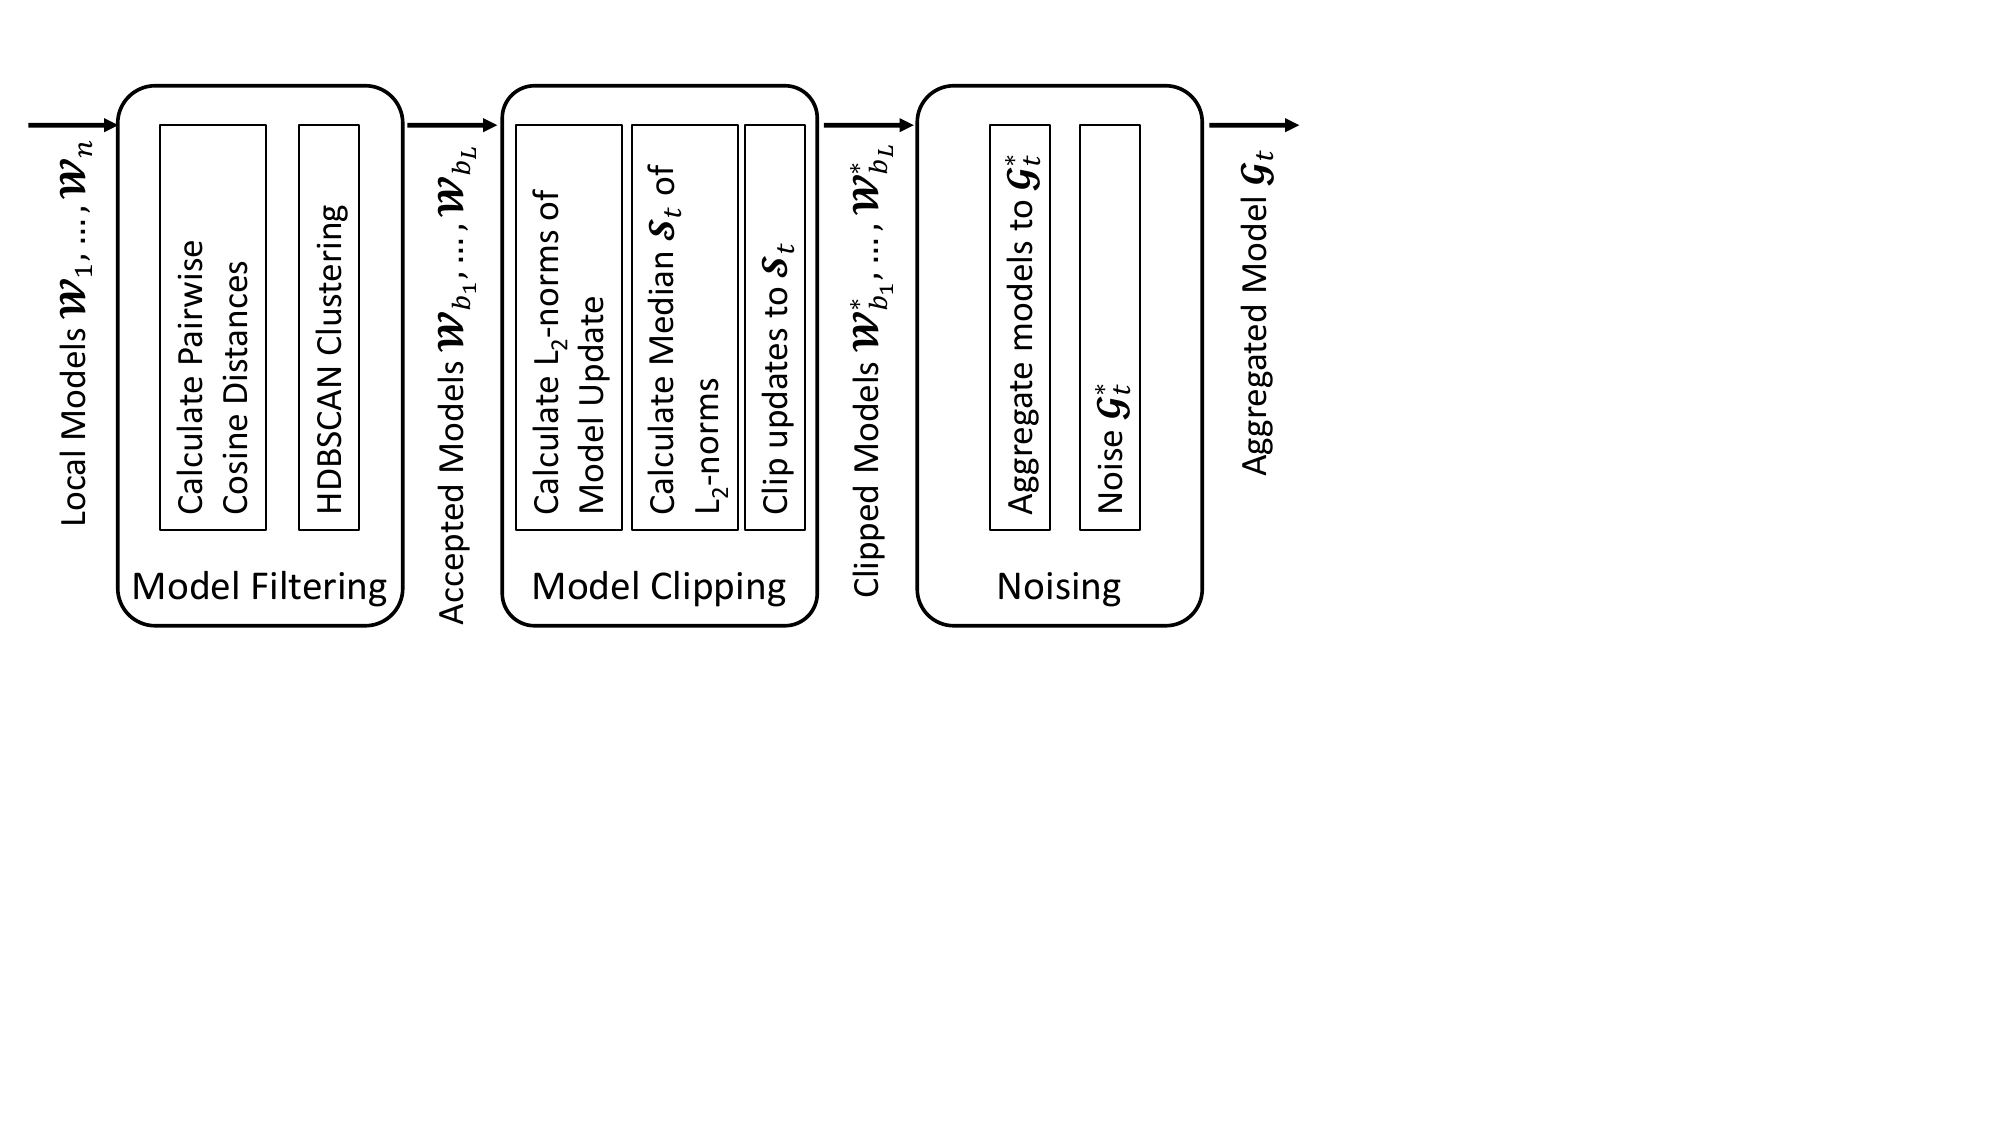}
    \caption{High-level overview of \flame.}
    \label{fig:flame}
\end{figure}
